# Supplementary material for: Bottom-Up Skill Discovery from Unsegmented Demonstrations for Long-Horizon Robot Manipulation
Source: arXiv:2109.13841 source file (2022-01-22)
Supplement: Supplementary file 1 [file supp.tex]

\section{Environments}
\label{sec:app-env}
% In \tooluse~ environment,  In \hammer~,. In \kitchen~, . These three environments require multi-stage execution and cover a large range of manipulation skills, ranging from prehensile skills to nonprehensile skills, and also from tool using to interaction with articulated objects. \multitask~ is a multitask domain designed for showing that we can discover reusable skills across different tasks. In \multitask domain,
\subsection{Task Descriptions}
We describe the execution stages that the robot needs to accomplish before reaching task goals in each environment.

\paragraph{\tooluse{} Task} The task goal is to put the cube into the metal pot. The robot needs to use the tool to fetch a cube which is not reachable for robot because the configuration for directly picking it up is almost at the singularity of robot's configuration. And after fetching, it needs to put the tool aside and put the cube into the pot.

\paragraph{\hammer{} Task} The task goal is to put the hammer in the drawer and close the drawer. For achieving this goal, the robot needs to open up the drawer, place the hammer into the drawer, and close the drawer. The hammer is small and hard to grasp stably. 

\paragraph{\kitchen{} Task} The robot's goal is to cook and serve a simple dish in the serving region and turn off the stove. For this goal, the robot has to complete multiple steps in a sequence: turn on the stove, place the pot on the stove, put the ingredient into the pot, put the pot on the table, push it to the serving region (red region on the table), and turn off the stove at the end. This contains more execution stages of contact-rich motion than \tooluse{} and \hammer{} do.

\paragraph{\multitask{} Domain} We design three tasks in this domain, each with a different manipulation goal. The manipulation goals are 1) \task{1}: The drawer is closed, the stove is turned on, the object is in the pot and the pot is placed on the stove; 2) \task{2}: The drawer is closed, the stove is turned on, the object is in the pot and the pot is in the serving region. 3) \task{3}: The drawer is closed, the stove cannot be turned on, the object is in the pot and the pot is in the serving region. And there are three sets of initial configuration for each task, which we visualize in Figure~\ref{fig:multitask-configs}.

% \task{1} has: 1) The stove is on, the object and the pot are on the table, the drawer is not closed and blocked the arm (Fig.~\ref{fig:multi-task-11}); 2) The stove is on, the object and the pot on the table, the drawer is closed (Fig.~\ref{fig:multi-task-12}) ; 3) The stove is off in the beginning, the object and the pot are on the table (Fig.~\ref{fig:multi-task-13}).
% \task{2} has: 1) The stove is off, the drawer is closed, the object and the pot are on the table, the drawer is closed (Fig.~\ref{fig:multi-task-21}) ; 2) The stove is on, the drawer is closed, the object and the pot are on the table (Fig.~\ref{fig:multi-task-22}); 3) The stove is on but the drawer is not closed, the object and the pot are on the table (Fig.~\ref{fig:multi-task-23}). 
% \task{3} has: 1) The drawer is open, the stove is off,  the pot is on the table and the object is already in the pot (Fig.~\ref{fig:multi-task-31}); 2) The drawer is closed, the stove is off, the object and the pot are on the table (Fig.~\ref{fig:multi-task-32}); 3) The drawer is open, stove turned off, the object and the pot are both on the table (Fig.~\ref{fig:multi-task-33}).

We collect $120$ demonstrations for each task. We collect the same number of demonstrations for all different sets of initial configurations. The demonstration sequences of tasks for \test{} present two characteristics. 1) For \task{1} and \task{2}, the sequences start from initial configurations in the other task of training data, thus having intersections in execution stages; 2) For \task{3}, the sequences are longer than any of the sequences for the task during training, so the approach needs to compose skills for longer execution stages. As we have seen from Table~\ref{tab:multitask}, the testing performance in \task{3} is lower than \task{1} and \task{2} due to this more challenging characteristic than the other two tasks.

\begin{figure}[t]
\begin{minipage}[t]{0.33\linewidth}
     \includegraphics[width=\linewidth,trim=0cm 0cm 0cm 5cm,clip]{figures/supp/MultitaskKitchenDomain_0.png}
        \vspace{-5mm}
       \subcaption{\scriptsize \task{1} Init Config 1}
       \label{fig:multi-task-11}
      \end{minipage}
\begin{minipage}[t]{0.33\linewidth}
     \includegraphics[width=\linewidth,trim=0cm 0cm 0cm 5cm,clip]{figures/supp/MultitaskKitchenDomain_4.png}
        \vspace{-5mm}
       \subcaption{\scriptsize \task{1} Init Config 2}
       \label{fig:multi-task-12}
      \end{minipage}
\begin{minipage}[t]{0.33\linewidth}
     \includegraphics[width=\linewidth,trim=0cm 0cm 0cm 5cm,clip]{figures/supp/MultitaskKitchenDomain_6.png}
        \vspace{-5mm}
       \subcaption{\scriptsize \task{1} Init Config 3 (\test{})}
       \label{fig:multi-task-13}
      \end{minipage}

\begin{minipage}[t]{0.33\linewidth}
     \includegraphics[width=\linewidth,trim=0cm 0cm 0cm 5cm,clip]{figures/supp/MultitaskKitchenDomain_2.png}
        \vspace{-5mm}
       \subcaption{\scriptsize \task{2} Init Config 1}
       \label{fig:multi-task-21}
      \end{minipage}
\begin{minipage}[t]{0.33\linewidth}
     \includegraphics[width=\linewidth,trim=0cm 0cm 0cm 5cm,clip]{figures/supp/MultitaskKitchenDomain_3.png}
        \vspace{-5mm}
       \subcaption{\scriptsize \task{2} Init Config 2}
       \label{fig:multi-task-22}
      \end{minipage}
\begin{minipage}[t]{0.33\linewidth}
     \includegraphics[width=\linewidth,trim=0cm 0cm 0cm 5cm,clip]{figures/supp/MultitaskKitchenDomain_5.png}
        \vspace{-5mm}
       \subcaption{\scriptsize \task{2} Init Config 3 (\test{})}
       \label{fig:multi-task-23}
      \end{minipage}

\begin{minipage}[t]{0.33\linewidth}
     \includegraphics[width=\linewidth,trim=0cm 0cm 0cm 5cm,clip]{figures/supp/MultitaskKitchenDomain_1.png}
        \vspace{-5mm}
       \subcaption{\scriptsize \task{3} Init Config 1}
       \label{fig:multi-task-31}
      \end{minipage}
\begin{minipage}[t]{0.33\linewidth}
     \includegraphics[width=\linewidth,trim=0cm 0cm 0cm 5cm,clip]{figures/supp/MultitaskKitchenDomain_7.png}
        \vspace{-5mm}
       \subcaption{\scriptsize \task{3} Init Config 2}
       \label{fig:multi-task-32}
      \end{minipage}
\begin{minipage}[t]{0.33\linewidth}
     \includegraphics[width=\linewidth,trim=0cm 0cm 0cm 5cm,clip]{figures/supp/MultitaskKitchenDomain_8.png}
        \vspace{-5mm}
       \subcaption{\scriptsize \task{3} Init Config 3 (\test{})}
       \label{fig:multi-task-33}
      \end{minipage}
    \vspace{-1mm}
    \caption{Screenshots of example initial configurations for three tasks in \multitask{}. Each row corresponds to a task, and left two figures in each row represent initial configurations are covered in \trainmulti{}, \trainsingle{}. Every set of initial configurations shown in the right figure of each row is covered in \test{}. ~\ref{fig:multi-task-11}: The stove is on, the object and the pot are on the table, the drawer is not closed and blocked the arm; ~\ref{fig:multi-task-12}: The stove is on, the object and the pot on the table, the drawer is closed; ~\ref{fig:multi-task-13}: The stove is off in the beginning, the object and the pot are on the table; ~\ref{fig:multi-task-21}: The stove is off, the drawer is closed, the object and the pot are on the table, the drawer is closed; ~\ref{fig:multi-task-22}: The stove is on, the drawer is closed, the object and the pot are on the table; ~\ref{fig:multi-task-23}: The stove is on but the drawer is not closed, the object and the pot are on the table; ~\ref{fig:multi-task-31}: The drawer is open, the stove is off,  the pot is on the table and the object is already in the pot; ~\ref{fig:multi-task-32}: The drawer is closed, the stove is off, the object and the pot are on the table; ~\ref{fig:multi-task-33}: The drawer is open, the stove is off, the object and the pot are both on the table. }
    \label{fig:multitask-configs}
    \vspace{-7mm}
\end{figure}

\paragraph{\realrobot} The robot needs to take away the lid of the pot, place the pot to the plate, pick up the tool, use the tool to push the pot along with the plate to the margin of the table, and place down the tool in the the end. This task covers versatile motions of prehensile grasping motion, non-prehensile pushing motion, and tool using on the real hardware. 
%The task is significantly harder than any of the simulation environments. 
For capturing visual images, we use Kinect Azure as the workspace camera, and Intel Realsense D435i as the eye-in-hand camera. We capture RGB images from the two cameras, and then scale images down to $128\times128$ as input to our models.

% \paragraph{Data collection Details} 

\paragraph{Environment Parameters} The maximum number of steps we set during evaluation varies based on the task difficulty. We set $1500$ for \tooluse{}, \hammer{}, $5000$ for \kitchen{}, $2500$ for tasks in \multitask{}, and $5000$ for \realrobot{}.

\section{Additional Experimental Analysis}

\paragraph{Reusable Skills in \multitask{} Domain} In Figure~\ref{fig:skill-percentage}, we use pie charts to show the percentage of the $8$ discovered skills in each of the \multitask{} tasks (We omit the number in the figure for clarity). As we mention in Sec.~\ref{sec:experiments}, most of the skills are indeed shared and reused across different tasks. And we also visualize sequences of two skills across all three tasks in the figure. As we can see from the visualization, similar skills with slightly different visual features (closing the drawer, but the stove is either on or off) are clustered in one skill, and it can improve the robustness of learned skills to visual variance in the inputs.   

\begin{figure}
\centering
  \begin{minipage}[t]{0.5\textwidth}
\makeatletter\def\@captype{figure}
  \includegraphics[width=1.0\linewidth,trim=0cm 0cm 0cm 0cm,clip]{figures/supp/Skill_Percentage.pdf}
  \caption{Percentage of skills in each task. We also visualize three sequences of skill segments correspond to Skill $2$ and Skill $5$. While segments of the same skill have some differences across the tasks, the overall semantic event the skills correspond to are consistent.}   
  \label{fig:skill-percentage}
  \end{minipage}
\end{figure}

\revised{\paragraph{Impact of different clustering algorithms} We offer additional experiments to show the comparison of k-means clustering and spectral clustering for classifying skills. We evaluate in \kitchen{} domain, and show the task success rate in Table~\ref{tab:clustering-comparison} using the two clustering algorithms while keeping the rest of the \ourmethod{} algorithms unchanged. We find that the switch from spectral clustering to k-means results in no significant performance differences. In comparison, the spectral clustering variant produces slightly better results.}

\begin{table}[h]
\centering
% \vspace{-1mm}
\caption{\label{tab:clustering-comparison} \revised{Success rate (\%) in \kitchen{} with different clustering algorithms}}  
\makeatletter\def\@captype{table}
   \resizebox{0.8\linewidth}{!}{  
  \begin{tabular}{lccc}
    \toprule
    \textbf{} & Spectral Clustering & K-means Clustering \\
    \midrule
    \kitchen~ & $72.0\pm4.0$ & $70.6\pm3.7$\\
    \bottomrule
  \end{tabular}
  }
  \end{table}

\section{Model Details}
\label{sec:app-models}

% \subsection{Multi-Sensory Fusion}
% \revised{A more detailed diagram of the fusion process can be found in Figure 2 of the cited work~\cite{lee2020making}. The fused representation is optimized over an adapted ELBO (evidence lower bound) loss from Equation (3, 4) in ~\cite{lee2020making}. A major difference is that we optimized over reconstructing the current states while Lee et al. optimized over reconstructing the next states. This different design choice came from the fact that their work focused on using the latent representation as inputs for policy learning which needs to encode future state information, while we focused on learning the statistical patterns of multi-sensory data at the current state.}

%  We use the same convolutional network structures as the models from \citet{lee2020making}, except that we do not have skip connections from the encoder to the decoder parts.  We choose $32$ for The latent dimension of the fused representation. For training the fusion model for each task, we use $1000$ training epochs, with a learning rate of $0.001$. batch size of 128. 

\subsection{Skill Segmentation}

\paragraph{Hyperparameters} We present the hyperparameters for the unsupervised clustering step. The maximum number of clusters for each task is: $6$ for \tooluse{} and \hammer{}, $8$ for \kitchen{} and \realrobot{}, $10$ for \multitask{}. And the stopping criteria of the bread-first search is the number of segments of mid-level segments are more than twice the maximum number of clusters. We also use a minimum length threshold to reject a small cluster, the number we choose is: $30$ for \tooluse{}, \realrobot{}, $35$ for \hammer{}, $20$ for \multitask{}. In this work, these values of hyperparameters are tuned heuristically , and how to extend to an end-to-end method is another future direction to look at.

\subsection{Sensorimotor Policies}

\paragraph{Implementation Details}
\ourmethod{} focuses on learning closed-loop sensorimotor skills. The input to each skill is the observations from robot sensors and the latent subgoal vector $\omega_{t}$. Specifically, the observations consist of two RGB images ($128 \times 128$) from the workspace camera and the eye-in-hand camera, and the proprioception of joint and gripper states. For encoding visual inputs, we use ResNet-18~\cite{he2016deep} as the visual encoder, followed by Spatial Softmax~\cite{finn2016deep} to extract keypoints of the feature maps. We then concatenate keypoints with proprioception (joint angles and past five frames of gripper states~\cite{zhang2018deep}), and concatenated vectors are passed through fully connected layers with LeakyReLU activation, outputting end-effector motor commands. The subgoal encoder $E_k$ is a ResNet-18 module with spatial softmax module, and $E_k$ only takes the image from the workspace camera of the subgoal state in demonstration data as inputs. The meta controller $\pi_{H}$ takes the image of current observation from the workspace camera as input, and the visual encoder in $\pi_{H}$ is also a ResNet-18 module. For all ResNet-18 modules, we remove the last two layers compared to the original design, giving us $4\times4$ feature maps. For low-level robot controllers, we use position-based Operational Space Controller (OSC)~\cite{khatib1987unified} with a binary controller for the parallel-jaw gripper, and the controllers take commands at $20$ Hz. During evaluation, we choose the meta controller to operate at $4$ Hz while sensorimotor skills operate at $20$ Hz. 

We choose the dimension for subgoal vector $\omega_t$ to be $32$, the number of 2D keypoints from the output of Spatial Softmax layer to be $64$. We choose $H=30$ for all single-task environments (Both simulation and real robots). We choose $H=20$ for the multitask environment  \multitask{}. This is because skills are relatively short in each task in \multitask{} domain compared to all single-task environments. 

\paragraph{Training Details}
 To increase the generalization ability of the model, we apply data augmentation~\cite{kostrikov2020image} to images for both training skills and meta controllers. To further increase the robustness of policies $\pi^{(k)}_{L}$, we also add some noise from Gaussian distribution with a standard deviation of $0.1$. 
 
 For all skills, we train for $2001$ epochs with a learning rate of $0.0001$, and the loss function we use is $\ell_{2}$ loss. We use two layers ($300$, $400$ hidden units for each layer) for the fully connected layers in all sing-task environments, while three layers ($300$, $300$, $400$) hidden units for each layer for fully connected layers in \multitask{} domain. For meta controllers, we train $1001$ epochs in all simulated single-task environments, $2001$ epochs in \multitask{} domain, and $3001$ epochs in \realrobot{}. For kl coefficients during cVAE training, we choose $0.005$ for \tooluse{}, \hammer{}, and $0.01$ for all other environments. 
